# Supplementary material for: Episode Adaptive Embedding Networks for Few-shot Learning
Source: arXiv:2106.09398 source file (2021-06-17)
Supplement: Supplementary file 1 [file appendix.tex]

\clearpage
\newcommand{\beginsupplement}{%
        \setcounter{table}{0}
        \renewcommand{\thetable}{S\arabic{table}}%
        \setcounter{figure}{0}
        \renewcommand{\thefigure}{S\arabic{figure}}%
        \setcounter{section}{1}
        \renewcommand\thesubsection{\thesection.\arabic{subsection}}%
}

\pagenumbering{arabic}

\section*{Supplementary Material}
\beginsupplement

\subsection{Details of datasets}
\begin{table*}[hbt!]
    \centering
    \begin{tabular}{ *{5}{M{0.19\textwidth}} }
    \hline
    Dataset & Images & Classes & Train-val-test split & Resolution \\
    \hline
    miniImageNet & 60000 & 100 & 64/16/20 & 84$\times$84\\
    tieredImageNet & 779165 & 608 & 351/97/160 & 84$\times$84\\
    CIFAR-FS & 60000 & 100 & 64/16/20 & 32$\times$32\\
    \hline
    \end{tabular}
      \caption{Details of datasets.}
    \label{table_split}
\end{table*}

\subsection{Architecture of generic embedding networks}\label{sec_arch}
The ConvNet-4 network has four convolutional blocks \cite{maml,prototypical}. Each block begins with a $3\times 3$ $2$D convolutional kernel, followed by a batch normalization layer, a $2\times 2$ max-pooling layer and a ReLU activation layer. 
The ResNet-12 network has been used in \cite{tadam,meta-trans,opt}. In our work, it has four residual blocks. Each residual block consists of three convolutional layers. A convolutional layer uses a $3\times 3$ convolutional kernel, followed by a batch normalization layer and an activation layer, in which the leaky relu function is used. The channels for the residual blocks are $64$, $128$, $256$, and $64$, respectively.

\subsection{Parameter settings}
\begin{table}[hbt!]
    \centering
   \begin{tabular}{M{0.3\textwidth} M{0.15\textwidth} M{0.25\textwidth} M{0.25\textwidth}}
    \hline
     Parameters & Backbone & Init learning rate  & Decay iterations \\
     
     %\multirow{ 2}{*}{Parameters} & \multirow{ 2}{*}{Backbone} & Init learn-  & Decay \\ &&ing rate & iterations \\
     \hline
    miniImageNet & \multirow{3}{*}{ConvNet-4} & 1e-3 & 10,000  \\ 
    tieredImageNet &  & 1e-3 & 25,000 \\
    CIFAR-FS && 5e-4& 20,000\\\hline
    miniImageNet & \multirow{2}{*}{ResNet-12} & 1e-4 & 10,000   \\
    tieredImageNet &  & 1e-4 & 10,000 \\
    \hline
       \end{tabular}
    \caption{Parameters used in the experiments.}
    \label{table_parameter}
\end{table}

\subsection{Classification accuracies with different classifiers and generic embedding networks}

\begin{table*}[t]
    \centering
    \begin{tabular}{M{0.2\textwidth} M{0.15\textwidth} M{0.15\textwidth} *{4}{M{0.12\textwidth}}}
    
    \hline
          Model &  Backbone & Dataset &5-way $1$-shot &5-way $5$-shot &10-way $1$-shot &10-way $5$-shot\\
          \hline\hline
TPN \cite{propagation} & ConvNet-4 & \multirow{3}{*}{miniImageNet} & 53.75 & 69.43 & 36.62 & 52.32\\
EA-TPN (ours) & ConvNet-4 &  & 84.01 & 84.43 & 50.73 & 54.85 \\
TPN$\star$ \cite{propagation} & ResNet-12 &  & 57.12 & 71.38 & 51.45 & 55.64\\
EA-TPN (ours) & ResNet-12 &  & 84.06 & 88.34 & 51.45 & 55.64\\ \hline
PROTO \cite{prototypical} & ConvNet-4 &\multirow{3}{*}{miniImageNet} & 46.14 & 65.77 & 32.88 & 49.29\\
EA-PROTO (ours) & ConvNet-4 & & 92.95 & 96.55 & 67.66 & 77.64\\
PROTO$\star$ \cite{prototypical} & ResNet-12 & & 54.21 & 71.05 & 36.87 & 54.51\\
EA-PROTO (ours)& ResNet-12 & & 93.67 & 96.87 & 70.08 & 77.78\\

\hline\hline
TPN \cite{propagation} &  ConvNet-4 & \multirow{3}{*}{tieredImageNet} & 57.53 & 72.85 & 40.93 & 59.17\\
EA-TPN (ours) & ConvNet-4 & & 86.50 & 91.55 & 60.01 & 65.27\\
TPN$\star$ \cite{propagation} & ResNet-12 & & 59.30 & 77.93 & 46.04 & 66.85\\
EA-TPN (ours)& ResNet-12  & & 89.52 & 92.62 & 63.61 & 68.39\\\hline
PROTO \cite{prototypical} & ConvNet-4 & \multirow{3}{*}{tieredImageNet}& 48.58 & 69.57 & 37.35 & 57.83\\
EA-PROTO (ours) & ConvNet-4 & & 92.65 & 96.69 & 70.16 & 82.59 \\
PROTO$\star$ \cite{prototypical} & ResNet-12 & & 54.47 & 74.90 & 42.23 & 65.54\\
EA-PROTO (ours)& ResNet-12  & & 91.56 & 97.02 & 74.50 & 83.34 \\
\hline
    \end{tabular}
      \caption{Classification accuracies with different classifiers and generic embedding networks, where $\star$ denotes that the experimental results are from our implementation.}
    \label{table_combine}
\end{table*}
